# Supplementary material for: Symmetry and reactivity of $\pi$-systems in electric and magnetic fields: a perspective from conceptual DFT
Source: arXiv:2402.15595 source file (2024-02-23)
Supplement: Supplementary file 1 [file anionden.tex]

\section{Electron densities of \ce{[H2CO]-} anion and density difference plots}

%  \subsection{Contour plots for the electron densities of \ce{[H2CO]-}}

    \begin{figure*}[h!]
      \centering
      \includegraphics[width=.95\linewidth]{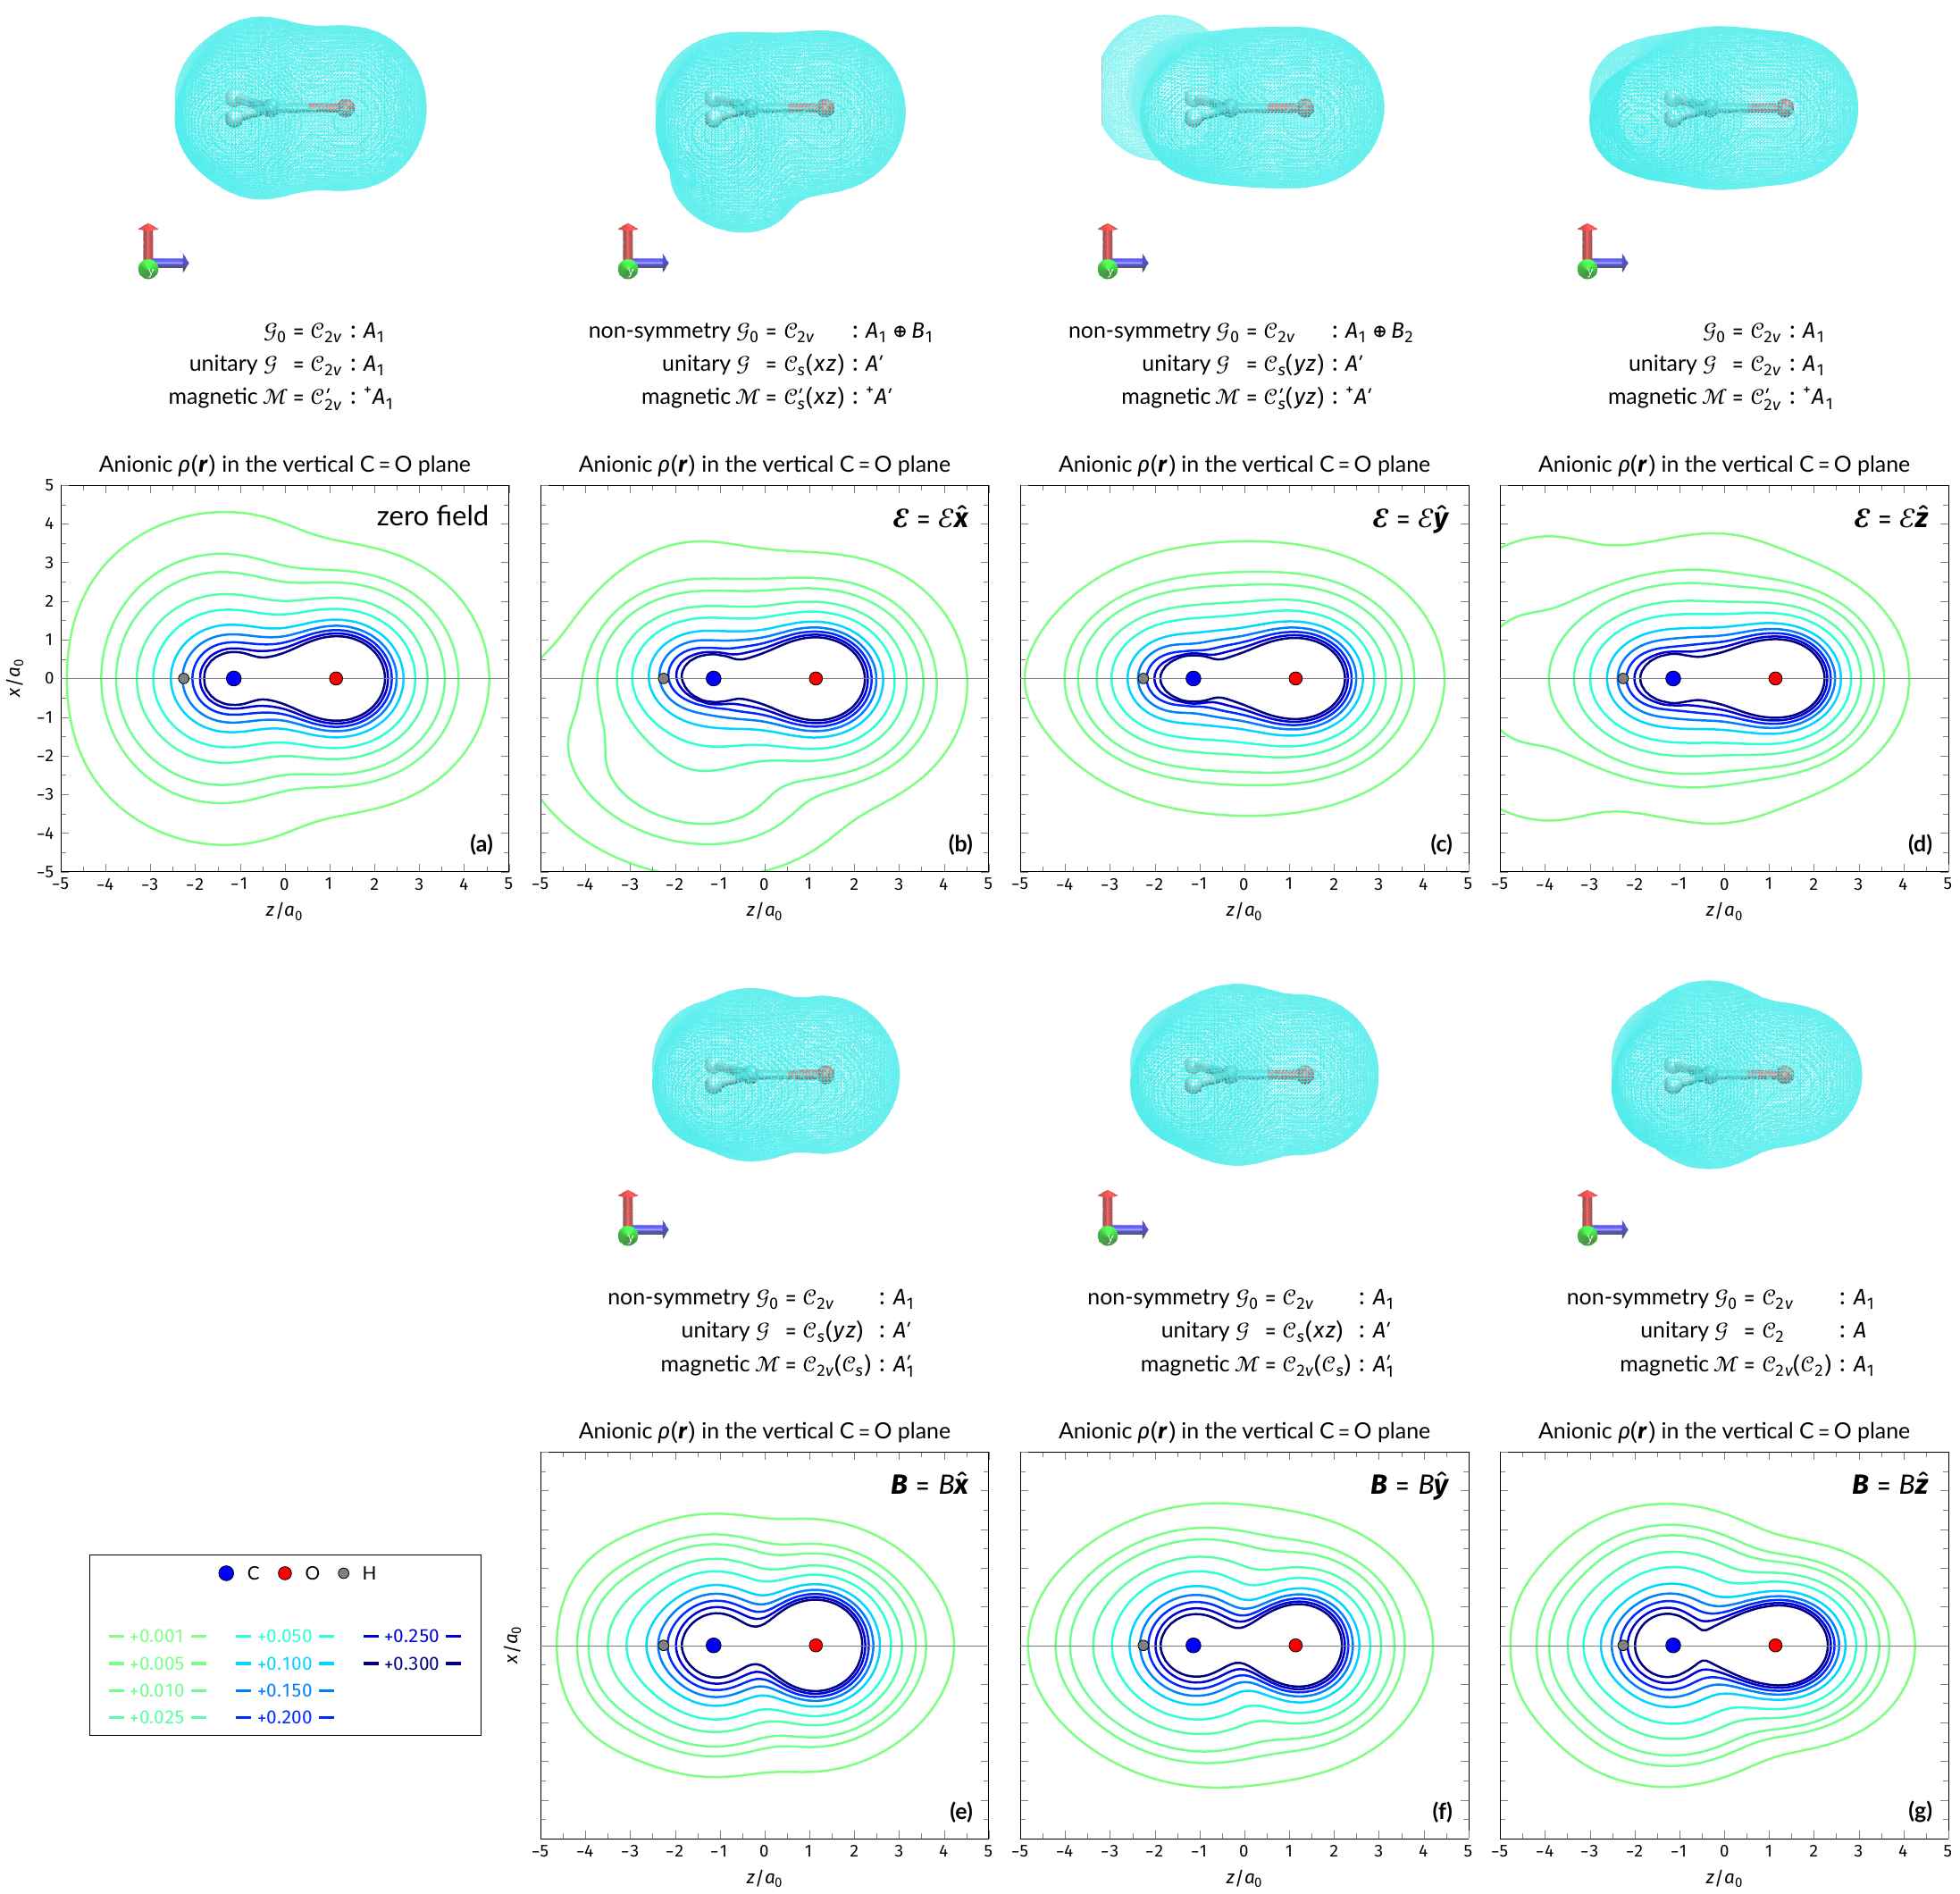}
      \caption{%
        Contour plots of the electron density $\rho(\mathbf{r})$ of the \ce{[H2CO]-} anion in various external-field configurations.
        Above each plot are the three-dimensional isosurface of the corresponding electron density at isovalue $\rho(\mathbf{r}) = 0.01$ and the representations spanned by $\rho(\mathbf{r})$ and its symmetry partners in various groups as determined by \qsymsq{} (see also Appendix~B in the main text for relevant character tables).
        Magnetic symmetries in $\mathcal{M}$ are given in terms of its  irreducible representations since electron densities are real-valued (\textit{cf.} Section~2.3.3.2 in the main text).
        All electron densities were calculated at the r\textsuperscript{2}SCAN0/cc-pVTZ level.
        The electric field strength $\mathcal{E}$ is set at \SI{0.1}{\atomicunit} and the magnetic field strength $B$ at $1.0 B_0$.
      }
      \label{fig:anion_densities}
    \end{figure*}

  \clearpage
%  \subsection{Contour plots for the electron densities of \ce{[H2CO]-}}

    \begin{figure*}[h!]
      \centering
      \begin{subfigure}{\textwidth}
        \centering
        \includegraphics[height=.8\textheight]{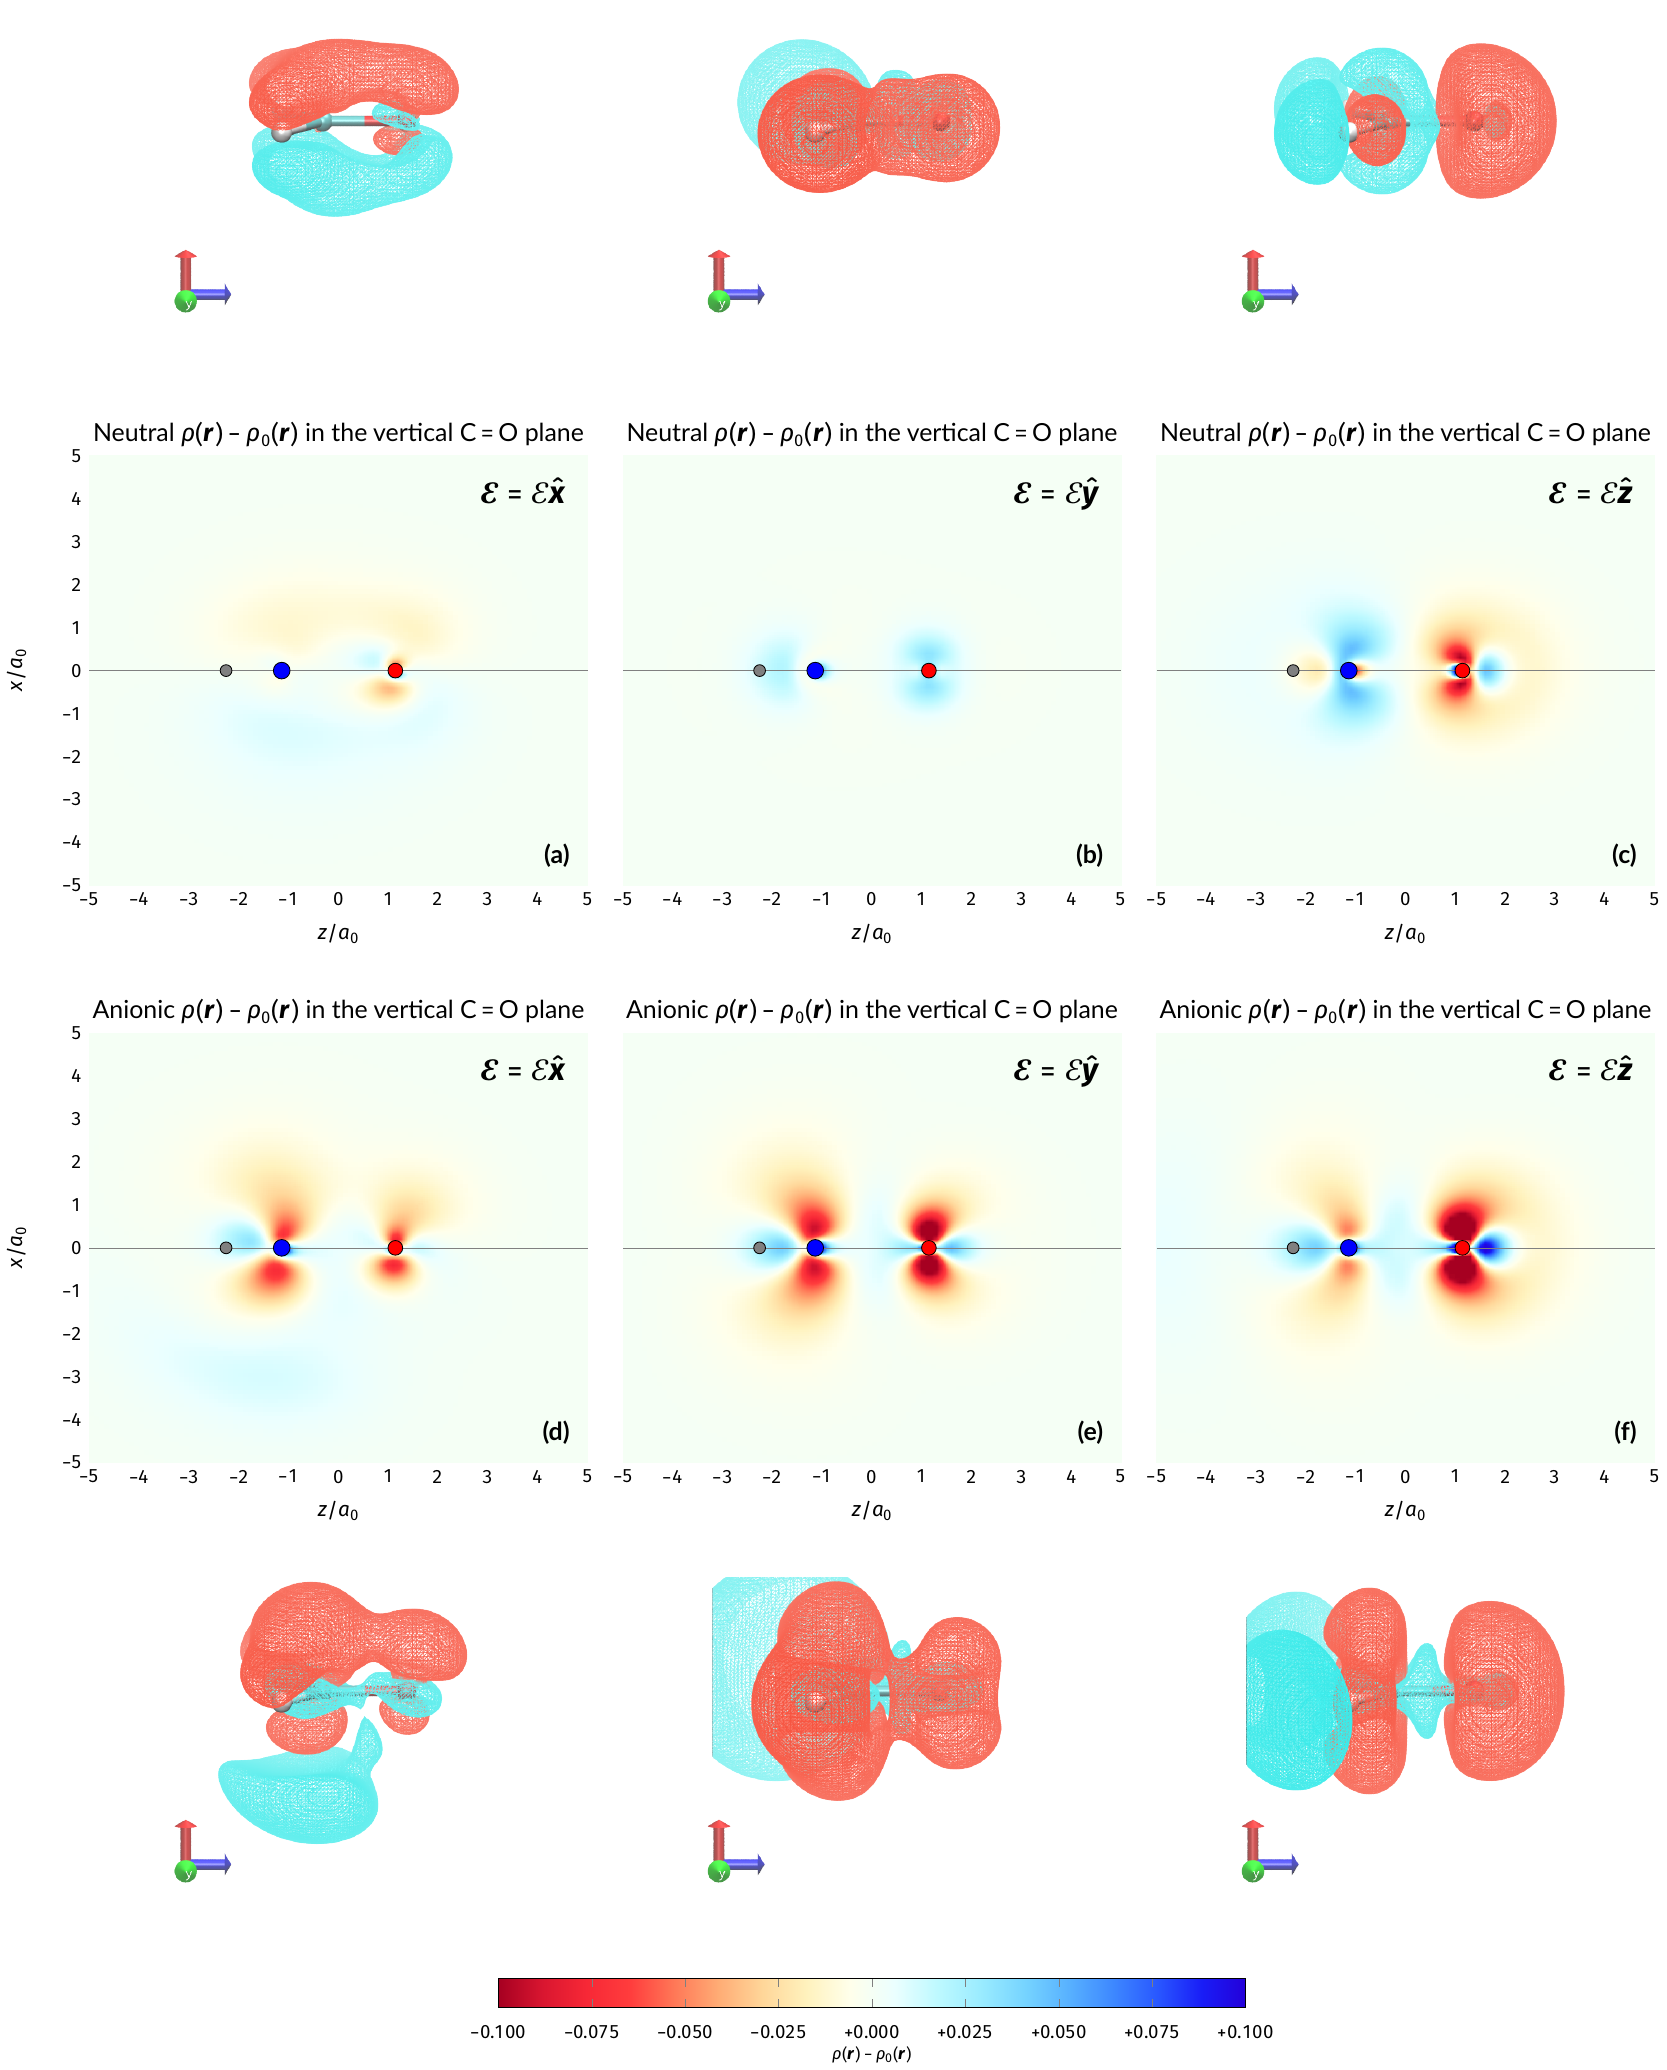}
        \caption*{(continued next page)}
      \end{subfigure}
    \end{figure*}

    \begin{figure*}[h!]
      \ContinuedFloat
      \begin{subfigure}{\textwidth}
        \centering
        \includegraphics[height=.8\textheight]{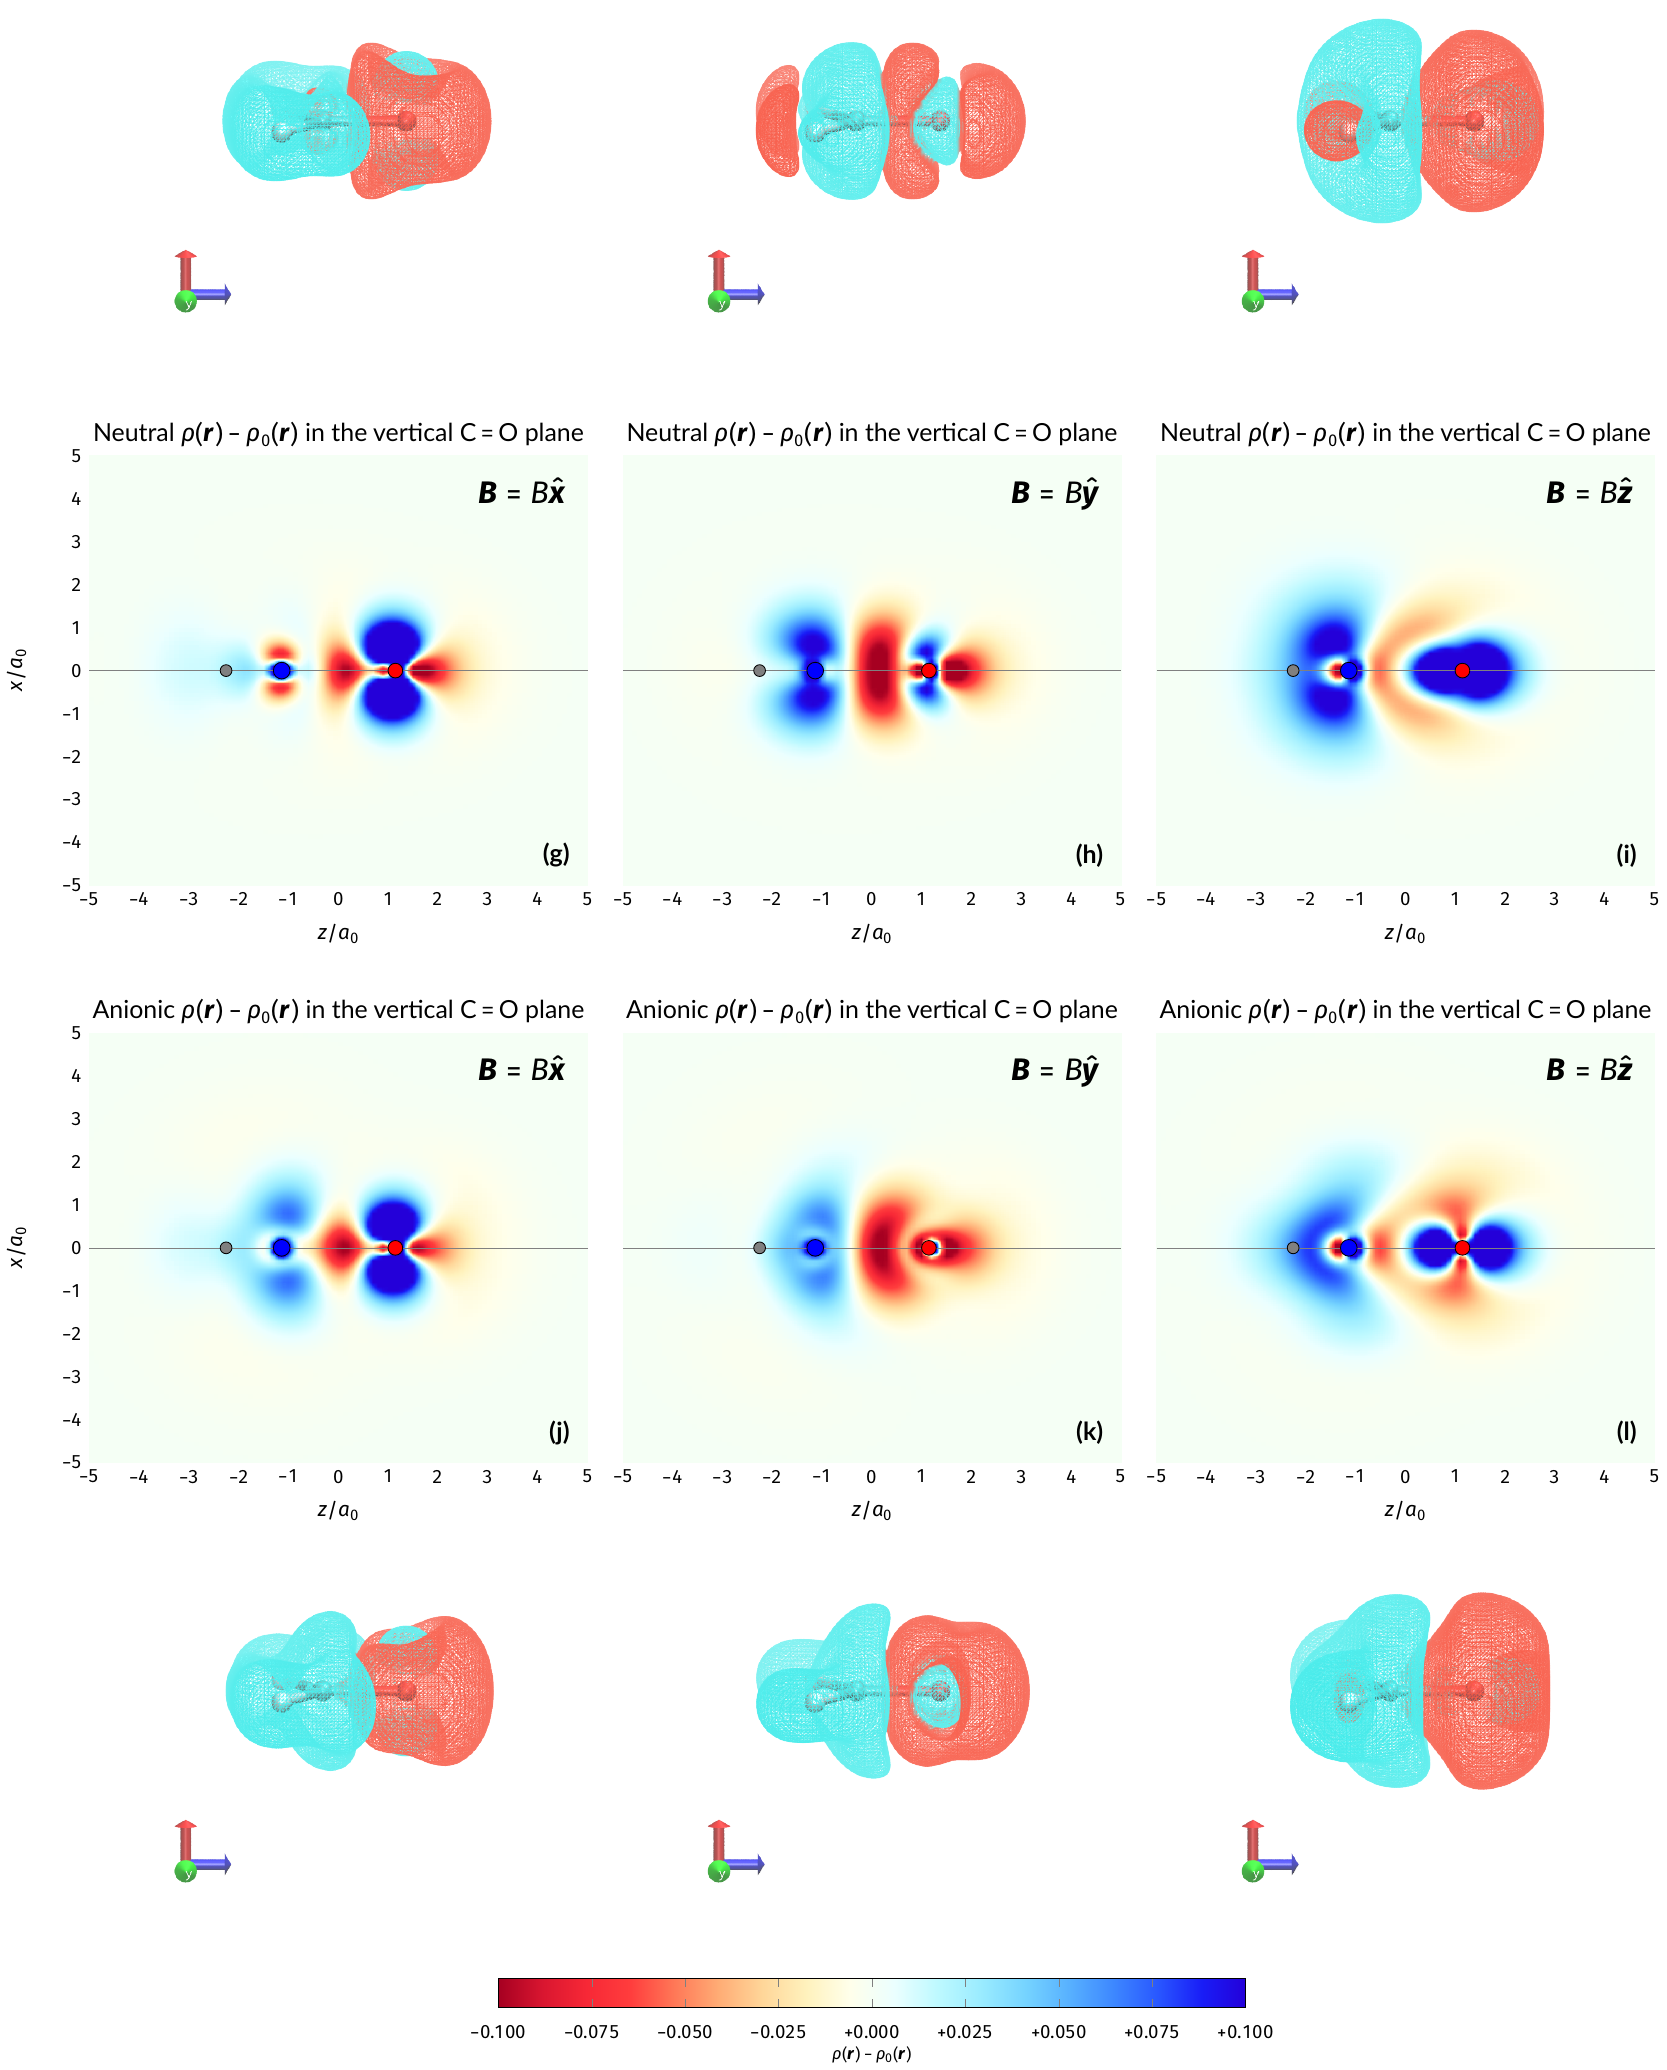}
      \end{subfigure}
      \caption{%
        Density difference plots in various external-field configurations.
        Each plot shows the difference $\rho(\mathbf{r}) - \rho_0(\mathbf{r})$ in the vertical \ce{C=O} plane with $\rho(\mathbf{r})$ the density of either the neutral species or the anionic one in the given field, and $\rho_0(\mathbf{r})$ the corresponding density at zero field.
        Each plot is also accompanied by an isosurface of the density difference shown at $\lvert \rho(\mathbf{r}) - \rho_0(\mathbf{r}) \rvert = 0.005$.
      }
      \label{fig:dendiff}
    \end{figure*}
