# Supplementary material for: Symmetry and reactivity of $\pi$-systems in electric and magnetic fields: a perspective from conceptual DFT
Source: arXiv:2402.15595 source file (2024-02-23)

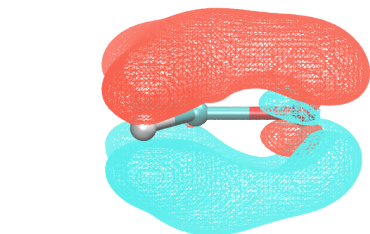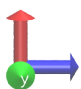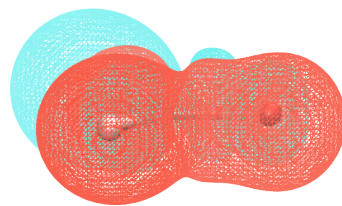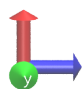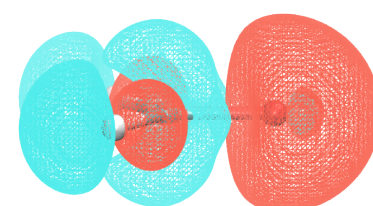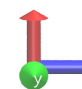

Neutral  $\rho(\mathbf{r}) - \rho_0(\mathbf{r})$  in the vertical C = O plane

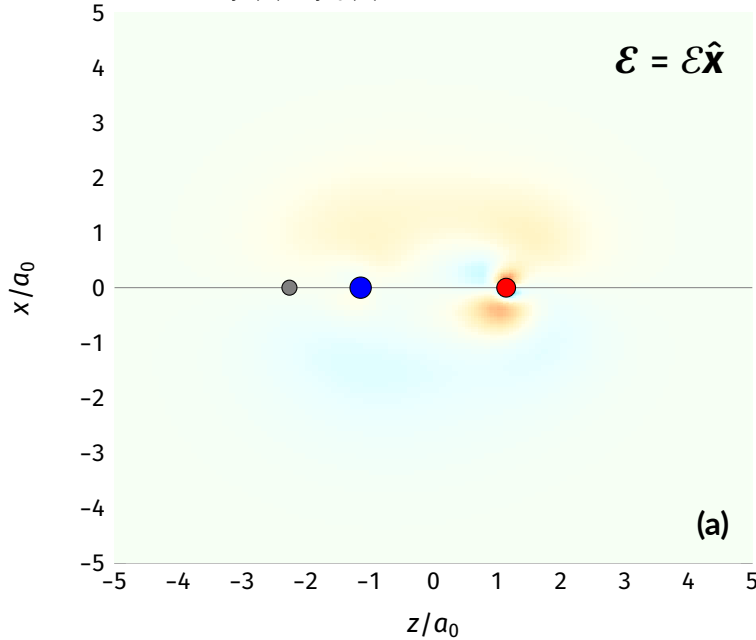

Neutral  $\rho(\mathbf{r}) - \rho_0(\mathbf{r})$  in the vertical C = O plane

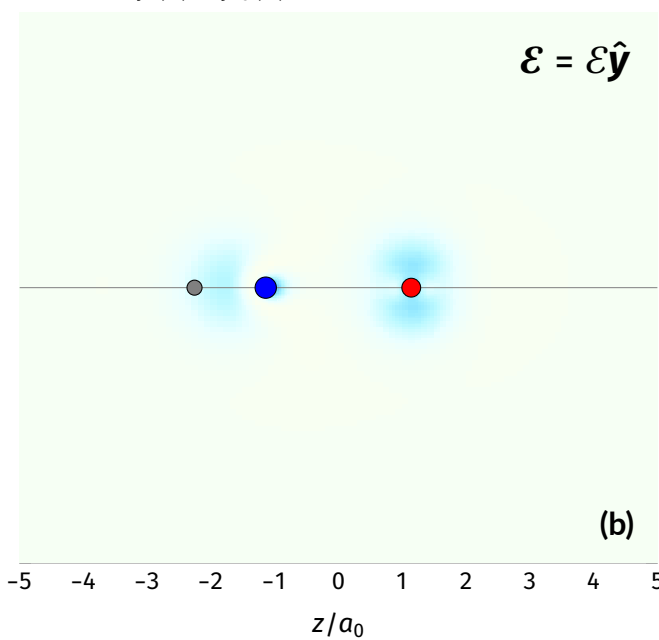

Neutral  $\rho(\mathbf{r}) - \rho_0(\mathbf{r})$  in the vertical C = O plane

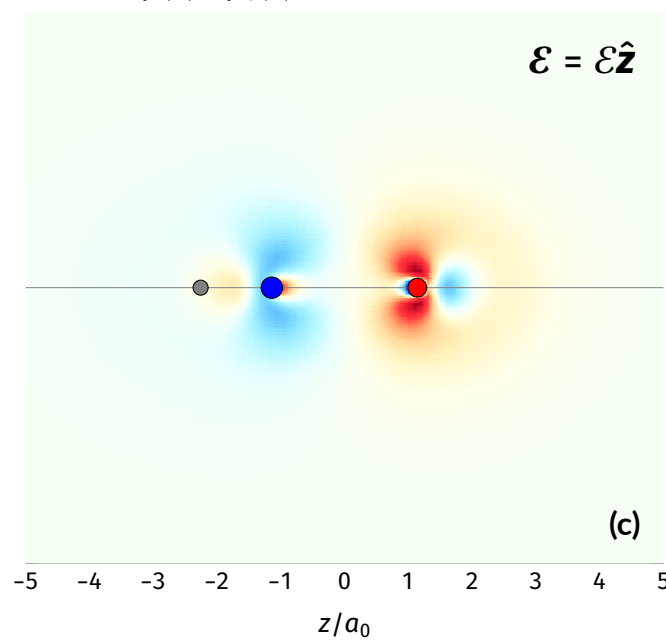

Anionic  $\rho(\mathbf{r}) - \rho_0(\mathbf{r})$  in the vertical C = O plane

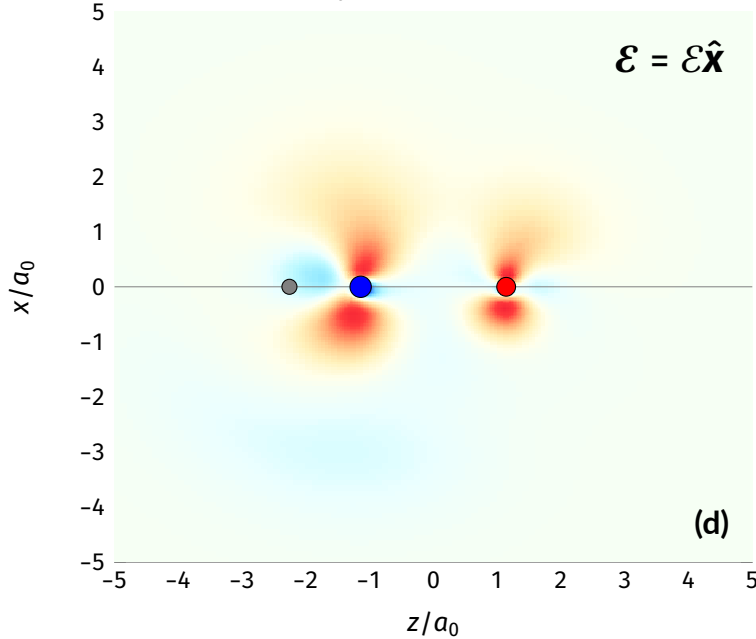

Anionic  $\rho(\mathbf{r}) - \rho_0(\mathbf{r})$  in the vertical C = O plane

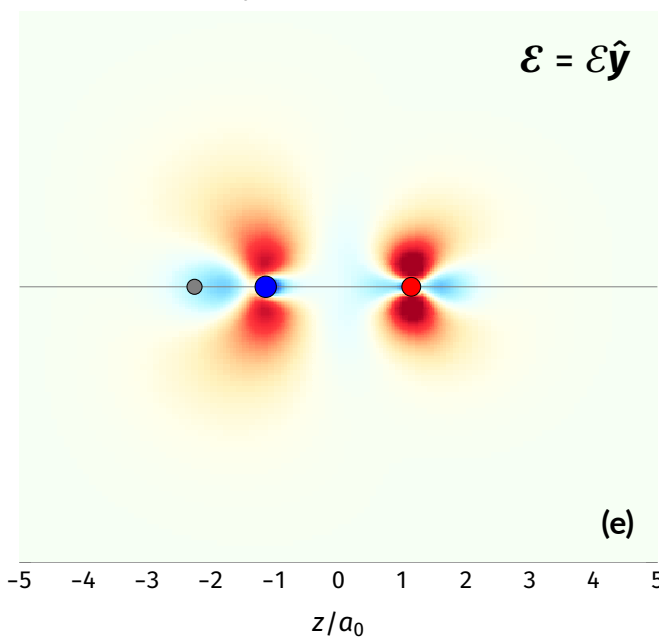

Anionic  $\rho(\mathbf{r}) - \rho_0(\mathbf{r})$  in the vertical C = O plane

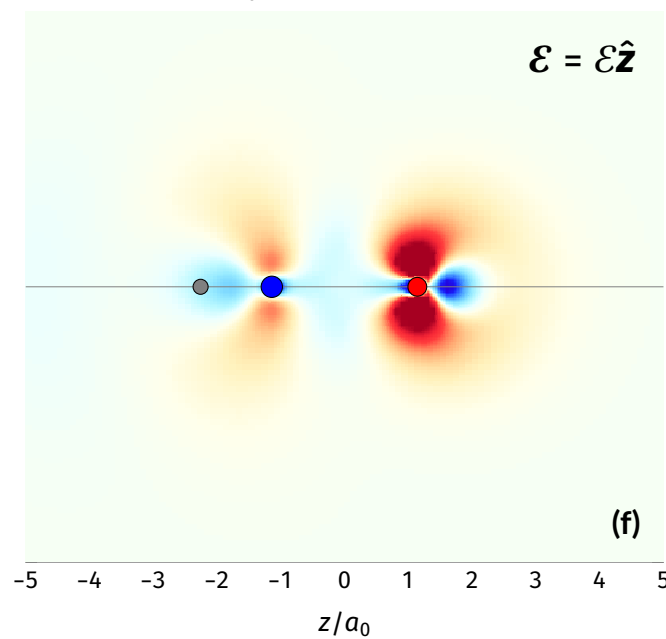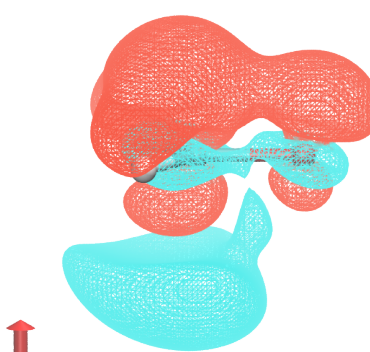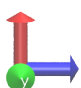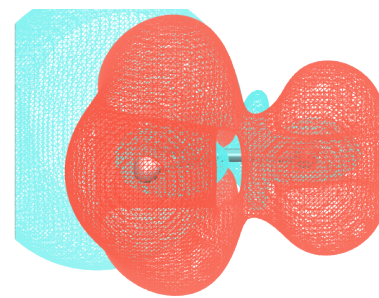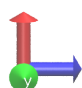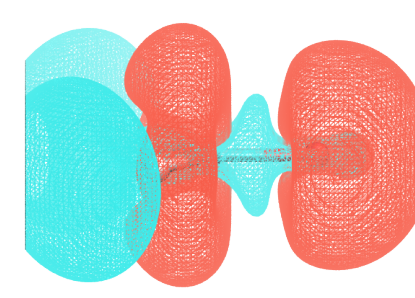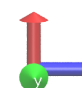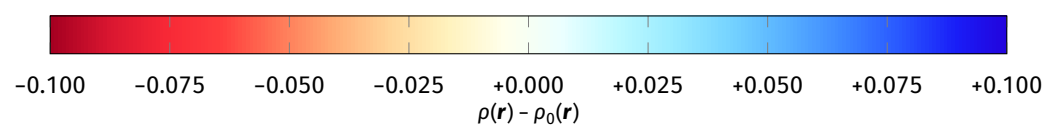

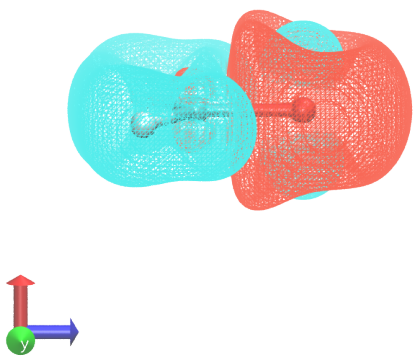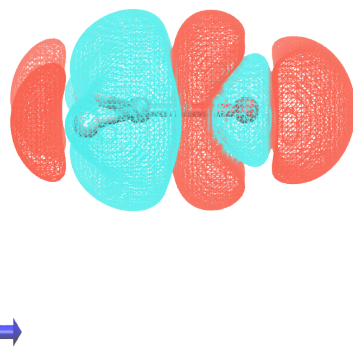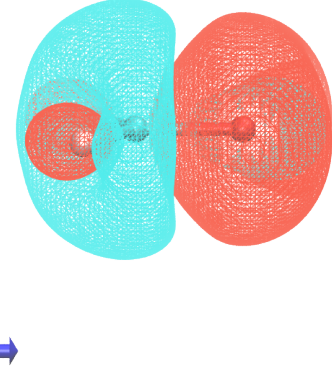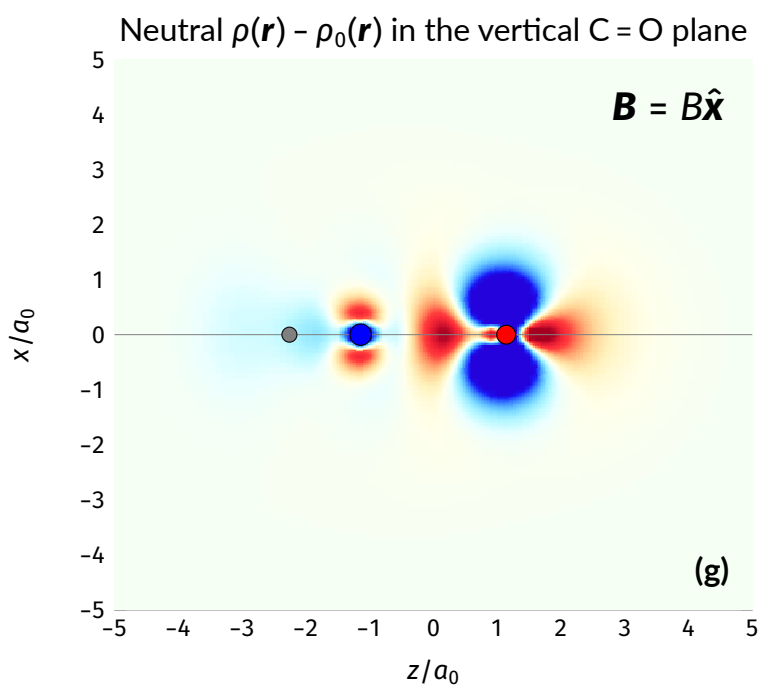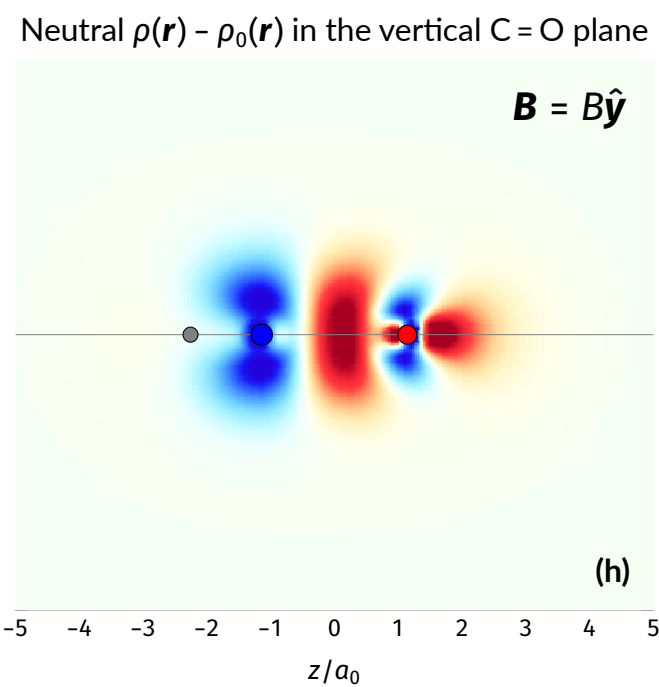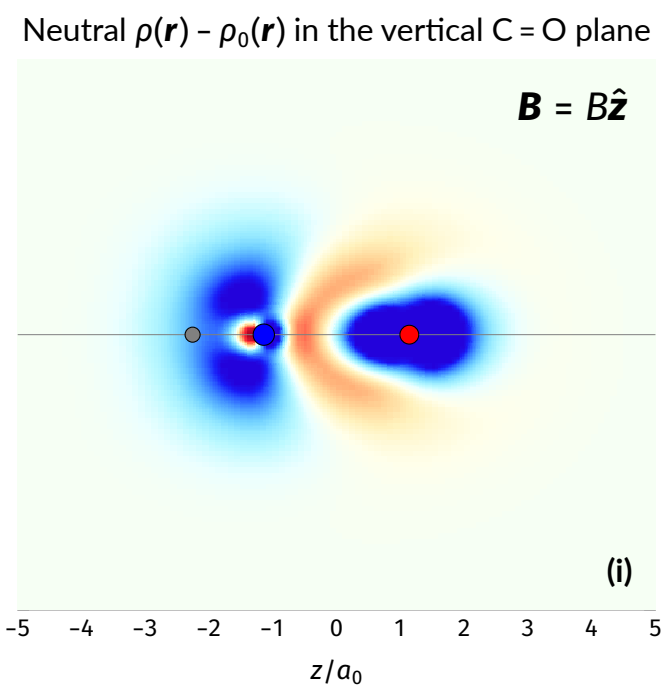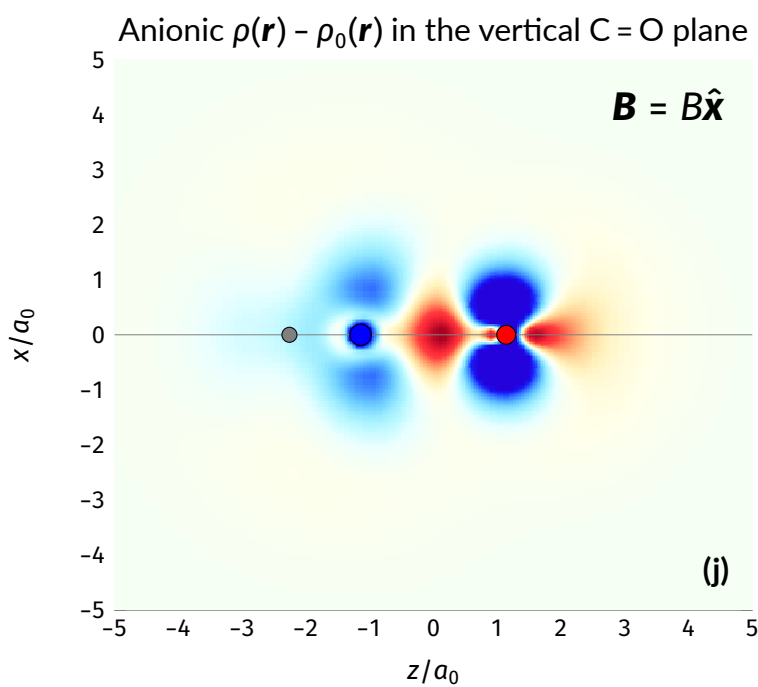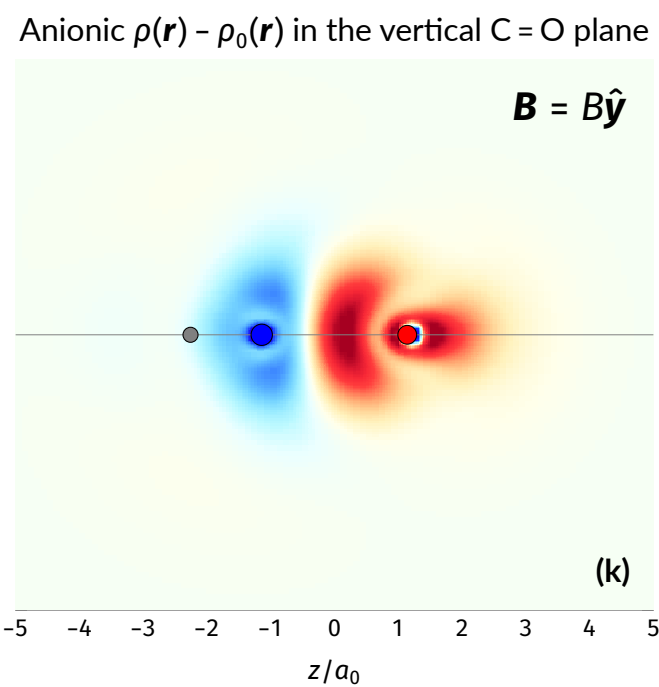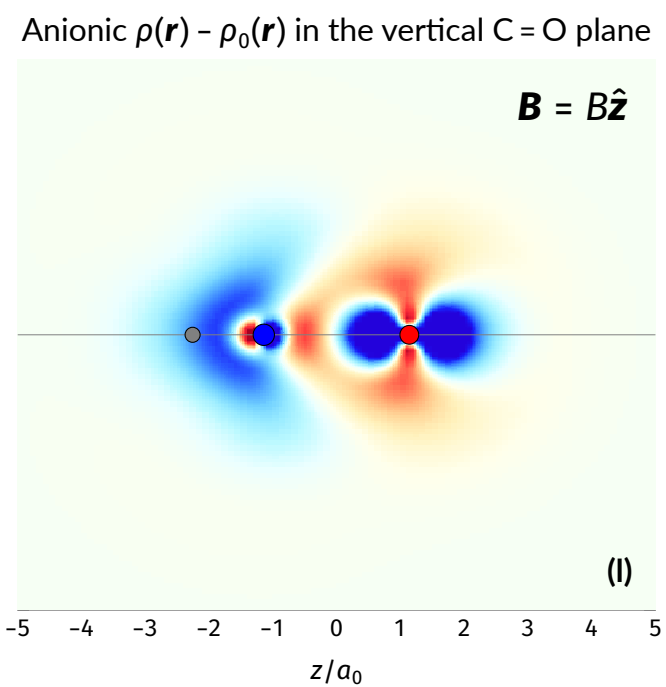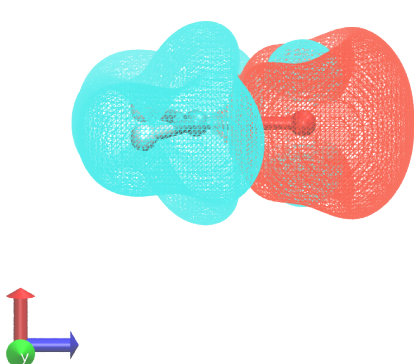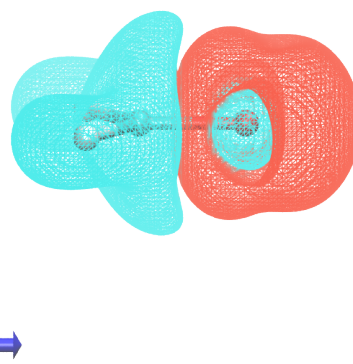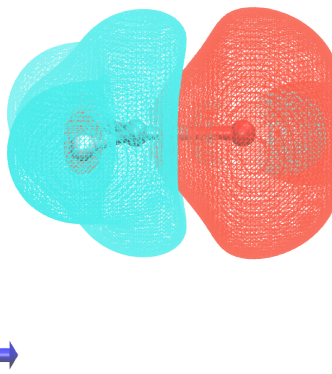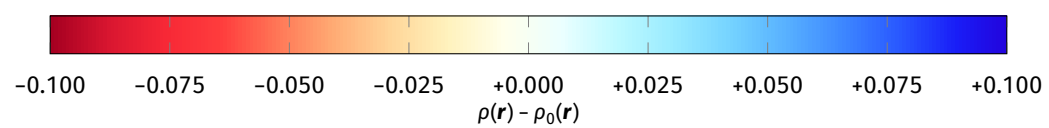

Supplement: Supplementary file 3 [file dendiff.pdf]
